# Supplementary material for: Neural Task Synthesis for Visual Programming
Source: arXiv:2305.18342 source file (2024-01-14)
Supplement: Supplementary file 1 [file fig_tutorcodes_overview.tex]

\begin{figure*}[h!]
\centering
    %%%%%%%%%%%%%%%%%    
    \begin{subfigure}[b]{.245\textwidth}
        \centering
		{
            %\begin{boxcode}{3.4cm}{0.80}{0.54}
   	    \begin{boxcode}{3.7cm}{0.75}{0.7}
                \textcode{def }\DSLRun\textcode{()\{}\\
                %\quad \DSLRepeatUntil\textcode{(}\DSLBoolGoal\textcode{)\{}\\
                %\quad \quad \DSLIf\textcode{(\DSLBoolPathLeft)}\textcode{\{}\\
                \quad \DSLRepeat\textcode{(3)\{}\\          
            	\quad \quad \DSLMove\\
                \quad \quad \DSLMove\\
                \quad \quad \DSLTurnRight\\
			    \quad \textcode{\}}\\
                \textcode{\}}
                \vspace{10mm}
            \end{boxcode}
    	}
        \vspace{-1.5mm}     
        \caption{$\code^{\text{out}}$ for $\spec_0$}
        \label{app-fig.tutors-code.spec0}
        \vspace{1mm}        
    \end{subfigure}    
    %
    %%%%%%%%%%%%%%%%%
    \begin{subfigure}[b]{.245\textwidth}
        \centering
        {
            %\begin{boxcode}{3.4cm}{0.80}{0.54}
   	        \begin{boxcode}{3.7cm}{0.75}{0.7}
                \textcode{def }\DSLRun\textcode{()\{}\\
                %\quad \DSLRepeatUntil\textcode{(}\DSLBoolGoal\textcode{)\{}\\
                %\quad \quad \DSLIf\textcode{(\DSLBoolPathLeft)}\textcode{\{}\\
                \quad \DSLRepeatUntil\textcode{(\DSLBoolGoal{})\{}\\ 
                \quad \quad \DSLTurnRight\\
            	\quad \quad \DSLMove\\
                \quad \DSLTurnLeft\\
                \quad \quad \DSLMove\\
			    \quad \textcode{\}}\\
                \textcode{\}}
                \vspace{7mm}
            \end{boxcode}
        }
        \vspace{-1.5mm}        
        \caption{$\code^{\text{out}}$ for $\spec_1$}
        \label{app-fig.tutors-code.spec1}
        \vspace{1mm}        
    \end{subfigure}
    %
    %%%%%%%%%%%%%%%%%
	\begin{subfigure}[b]{.245\textwidth}
        \centering
        {
            %\begin{boxcode}{3.4cm}{0.80}{0.54}
   	    \begin{boxcode}{3.7cm}{0.75}{0.7}
                \textcode{def }\DSLRun\textcode{()\{}\\
                \quad \DSLRepeat\textcode{(4)\{}\\          
            	\quad \quad \DSLMove\\
			    \quad \textcode{\}}\\
                \quad \quad \DSLTurnLeft\\
                \quad \DSLRepeat\textcode{(5)\{}\\          
            	\quad \quad \DSLMove\\
			    \quad \textcode{\}}\\
                \textcode{\}}
                \vspace{3.8mm}
            \end{boxcode}
    	}
        \vspace{-1.5mm}     
        \caption{$\code^{\text{out}}$ for $\spec_2$}
        \label{app-fig.tutors-code.spec2}   
        \vspace{1mm}
    \end{subfigure}
    %
    %%%%%%%%%%%%%%%%%
	\begin{subfigure}[b]{.245\textwidth}
	\centering
        {
            %\begin{boxcode}{3.4cm}{0.80}{0.54}
   	    \begin{boxcode}{3.7cm}{0.75}{0.7}
		      \textcode{def }\DSLRun\textcode{()\{}\\
                \quad \DSLRepeatUntil\textcode{(\DSLBoolGoal{})\{}\\
                \quad \quad \DSLIf\textcode{(\DSLBoolPathAhead{})\{}\\                
            	\quad \quad \quad \DSLMove\\
                \quad \quad \textcode {\}}\\
                \quad \quad \DSLElse \textcode{\{}\\
                \quad \quad \quad \DSLTurnLeft\\
                \quad\quad\textcode{\}}\\
			    \quad \textcode{\}}\\
		      \textcode{\}}
               % \vspace{1mm}
            \end{boxcode}
    	}
        \vspace{-1.5mm}     
        \caption{$\code^{\text{out}}$ for $\spec_3$}
        \label{app-fig.tutors-code.spec3}
        \vspace{1mm}
    \end{subfigure}
    \\
    %%%%%%%%%%%%%%%%%
    	\begin{subfigure}[b]{.245\textwidth}
        \centering
		{
            %\begin{boxcode}{3.4cm}{0.80}{0.54}
   	    \begin{boxcode}{3.7cm}{0.75}{0.7}
		      \textcode{def }\DSLRun\textcode{()\{}\\
                \quad \DSLRepeatUntil\textcode{(\DSLBoolGoal{})\{}\\
                \quad \quad \DSLMove\\
                \quad \quad \DSLIf\textcode{(\DSLBoolPathLeft{})\{}\\                
            	\quad \quad \quad \DSLTurnLeft\\
                \quad \quad \textcode {\}}\\
                \quad \quad \DSLIf\textcode{(\DSLBoolPathRight{})\{}\\  
                \quad \quad \quad \DSLTurnRight\\
                \quad\quad\textcode{\}}\\
			    \quad \textcode{\}}\\
		      \textcode{\}}
            \vspace{8mm}
            \end{boxcode}
    	}
        \vspace{-1.5mm}     
        \caption{$\code^{\text{out}}$ for $\spec_4$}
        \label{app-fig.tutors-code.spec4}
        \vspace{1mm}        
    \end{subfigure}    
    %
    %%%%%%%%%%%%%%%%%
    \begin{subfigure}[b]{.245\textwidth}
        \centering
        {
            %\begin{boxcode}{3.4cm}{0.80}{0.54}
            \begin{boxcode}{3.7cm}{0.75}{0.7}
                \textcode{def }\DSLRun\textcode{()\{}\\
                \quad \DSLMove\\
                \quad \DSLMove\\
                \quad \DSLPutMarker\\
                \quad \DSLMove\\
                \quad \DSLMove\\
		      \textcode{\}}
            \vspace{22.3mm}
		  \end{boxcode}
        }
        \vspace{-1.5mm}        
        \caption{$\code^{\text{out}}$ for $\spec_5$}
        \label{app-fig.tutors-code.spec5}
        \vspace{1mm}        
    \end{subfigure}
    %
    %%%%%%%%%%%%%%%%%
	\begin{subfigure}[b]{.245\textwidth}
        \centering
        {
            %\begin{boxcode}{3.4cm}{0.80}{0.54}
   		\begin{boxcode}{3.7cm}{0.75}{0.7}
		      \textcode{def }\DSLRun\textcode{()\{}\\
                \quad \DSLPutMarker\\
                \quad \DSLWhile\textcode{(\DSLBoolPathAhead)\{}\\
            	\quad \quad \DSLMove\\
            	\quad \quad \DSLTurnLeft\\
            	\quad \quad \DSLMove\\
            	\quad \quad \DSLTurnRight\\
            	\quad \quad \DSLPutMarker\\
			    \quad \textcode{\}}\\
		      \textcode{\}}
            \vspace{12.3mm}
            \end{boxcode}
    	}
        \vspace{-1.5mm}     
        \caption{$\code^{\text{out}}$ for $\spec_6$}
        \label{app-fig.tutors-code.spec6}       
        \vspace{1mm}
    \end{subfigure}
    %
    %%%%%%%%%%%%%%%%%
	\begin{subfigure}[b]{.245\textwidth}
	\centering
        {
            %\begin{boxcode}{3.4cm}{0.80}{0.54}
   		\begin{boxcode}{3.7cm}{0.75}{0.7}
			 \textcode{def }\DSLRun\textcode{()\{}\\
                \quad \DSLWhile\textcode{(\DSLBoolPathAhead{})\{}\\
            	\quad \quad \DSLPickMarker{} \\
            	\quad \quad \DSLMove{} \\
                \quad \textcode {\}}\\
            	\quad \DSLPickMarker{} \\
                \quad \DSLTurnLeft{}\\
                \quad \DSLTurnLeft{}\\
                \quad \DSLWhile\textcode{(\DSLBoolPathAhead{})\{}\\
            	\quad \quad \DSLMove{} \\
                \quad \textcode {\}}\\
                \quad \DSLTurnLeft{}\\
                \quad \DSLTurnLeft{}\\         
			 \textcode{\}}
		   \end{boxcode}
    	}
        \vspace{-1.5mm}     
        \caption{$\code^{\text{out}}$ for $\spec_7$}
        \label{app-fig.tutors-code.spec7}
        \vspace{1mm}
    \end{subfigure}
    	\begin{subfigure}[b]{.245\textwidth}
        \centering
		{
            %\begin{boxcode}{3.4cm}{0.80}{0.54}
   		\begin{boxcode}{4.2cm}{0.75}{0.7}
			 \textcode{def }\DSLRun\textcode{()\{}\\
                \quad \DSLWhile\textcode{(\DSLBoolNoPathAhead{})\{}\\
                \quad \quad \DSLIf\textcode{(\DSLBoolMarkerPresent{})\{}\\
            	\quad \quad \quad \DSLPickMarker{} \\
                \quad \quad \textcode {\}}\\
                \quad \quad \DSLTurnLeft{}\\
                \quad \quad \DSLMove{}\\
                \quad \quad \DSLTurnRight{}\\
                \quad \quad \DSLMove{}\\                
			    \quad \textcode{\}}\\
			 \textcode{\}}
		   \end{boxcode}
    	}
        \vspace{-1.5mm}     
        \caption{$\code^{\text{out}}$ for $\spec_8$}
        \label{app-fig.tutors-code.spec8}
        \vspace{1mm}        
    \end{subfigure}    
    %
    %%%%%%%%%%%%%%%%%
    \begin{subfigure}[b]{.245\textwidth}
        \centering
        {
            %\begin{boxcode}{3.4cm}{0.80}{0.54}
   		\begin{boxcode}{3.7cm}{0.75}{0.7}
		          \textcode{def }\DSLRun\textcode{()\{}\\
                    \quad \DSLPutMarker\\
                    \quad \DSLWhile\textcode{(\DSLBoolPathAhead)\{}\\
                    \quad \quad \DSLRepeat\textcode{(8)\{}\\
                    \quad \quad \quad \DSLPickMarker\\
                    \quad \quad \textcode {\}}\\
                	\quad \quad \DSLMove\\
    			    \quad \textcode{\}}\\
    		    \textcode{\}}
                \vspace{5.5mm}
                \end{boxcode}
    	}
        \vspace{-1.5mm}        
        \caption{$\code^{\text{out}}$ for $\spec_9$}
        \label{app-fig.tutors-code.spec9}
        \vspace{1mm}        
    \end{subfigure}
    %
    %%%%%%%%%%%%%%%%%
    \caption{Codes {\scriptsize $\AlgoTutor$}}
    \label{app-fig.tutors-code}
\end{figure*}
