# Supplementary material for: Neural Task Synthesis for Visual Programming
Source: arXiv:2305.18342 source file (2024-01-14)
Supplement: Supplementary file 2 [file fig_codegen_training_hyperparams.tex]

% !TEX root =  main.tex
%%%%%%%%%%%%%%%%%%%%%%%%%%%%%%%%%%%
%%%%%%%%%%%%%%%%%%%%%%%%%%%%%%%%%%%
\begin{figure*}[h!]
\centering
    \scalebox{0.9}{
        \setlength\tabcolsep{2.5pt}
        
        \begin{tabular}{c|c c}     
            \hline
            HyperParameter & \hocType{} & \karelType \\
            \hline
            Max. Epochs & $60$ & $100$ \\
            Batch Size & $32$ & $32$ \\
            Learning Rate & $5\times10^{-4}$ & $5\times10^{-4}$\\
            Dict. Size & $59$ & $59$ \\
            Max. Blocks & $17$ & $17$ \\
            \hline   
        \end{tabular}
        }
    \caption{Table containing the hyperparameters for the neural model for the code generator for each of the \hocType{} and \karelType{} domains.}
    \label{app-fig.hyperparams.codegen}
    %%%%%%%%%%%%%%%%%
\end{figure*}

%%%%%%%%%%%%%%%%%%%%%%%%%%%%%%%%%%%
%%%%%%%%%%%%%%%%%%%%%%%%%%%%%%%%%%%
